# Supplementary material for: Strange nonchaos in self-excited singing flames
Source: arXiv:1910.06916 source file (2019-10-09)
Supplement: Supplementary file 1 [file supple.pdf]

# Strange nonchaos in self-excited singing flames

D. Premraj[1], Samadhan A. Pawar[1], Lipika Kabiraj[2], R. I. Sujith[1]
[1]*Department of Aerospace Engineering, Indian Institute of Technology Madras, Chennai 600 036, India*
[2]*Department of Mechanical Engineering, Indian Institute of Technology Ropar, Punjab 140 001, India*
( Dated: September 15, 2019; Received : to be included by reviewer)

Here we provide details of our fractal dimension and self similarity calculations for the thermoacoustic system. These metrics can support other evidence for strange nonchaotic dynamics.

## I. FRACTAL DIMENSION

Fractals are geometric complex patterns which shows the self-similarity across different scales. The term fractal was first introduced by Benoit Mandelbrot (1982) to describe non-Euclidean structures that show self-similarity at different scales. Measures such as length and area of fractal are dependent upon the scale at which the fractal is measured. The log-log plot of the fractal measures (length and area) using the scaling factor (scales of measurement) gives a straight line with negative slope. The negative slope is termed as the fractal dimension (FD). Most of the natural features which show discontinuities and fragmentation tend to have a fractal dimension (Al-Kadi & Watson 2008). Also, most of these natural structures are complicated and rarely have an exact Euclidean (smooth) shape so that they can be precisely measured. The fractal dimension offers the ability to describe and characterize these structures. The fractal path for the cosidered system is shown in Fig. 1(a) which clearly delineates the complex pattern in $(Re(x), Im(x))$ plane.

So far in the literature, various algorithms are computed to identify the fractal dimension including exact algorithm (Clark 1986), hybrid algorithm (Turner et al. 1998), box-counting algorithm (Mandelbrot 1982) and differential box-counting algorithm (Sarkar & Chaudhuri 1993) etc. The differential box-counting algorithm is considered as an optimal method to estimate the fractal dimension of a gray scale image (Sarkar & Chaudhuri 1993, Napolitano *et al.* 2012). Hence, we use the differential box counting method to estimate the fractal dimension of the turbulent flame. The general expression for fractal dimension (FD) is

$$FD = \frac{\log n(r)}{\log r} \tag{1}$$

where $n(r)$ is the total number of boxes which cover the total image and $r$ is the length of the box edge. From Fig. 1(b), it is clear that the number of boxes decreases with increasing the length of boxes and fractal dimension is obtained as $FD = -1.63 \pm 0.105$.

## II. SELF-SIMILARITY OF SNA

The spectral random walk corresponds to fractal object on the $(Re(x),\ Im(x))$ plane show Fig. 2(a). Graphs at at suitably adjusted times (correspomding to the Fig. 2(a)) show a self-similar walk in the Fig. 3. From the spectrum of SNA, it is evident that for different time scales, the spectrum shows self similar dynamical effects which confirms the fractal nature of SNA.

[1] P. Grassberger and I. Procaccia, Phys. D, **9**, 189 (1983).

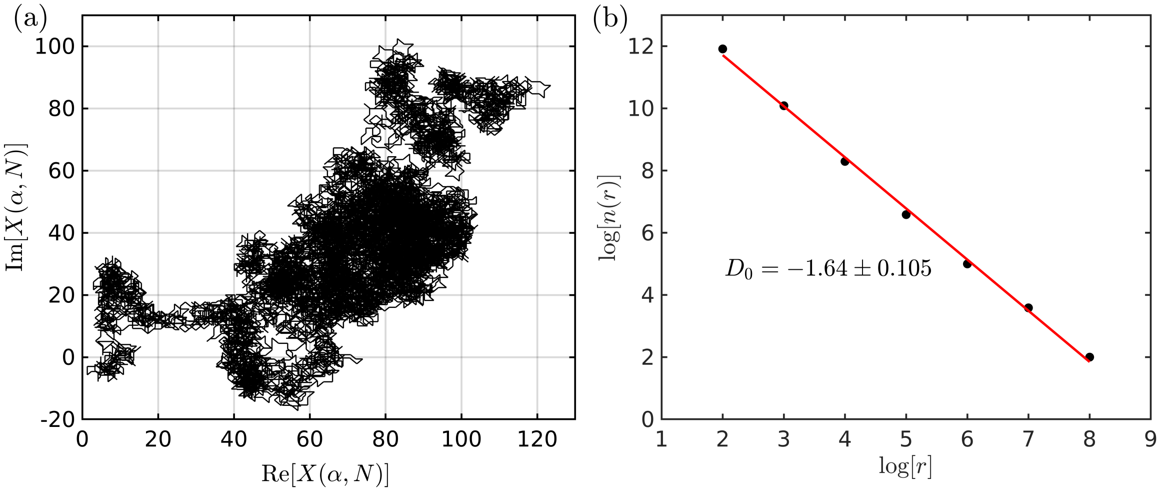


FIG. 1. (a) Fractal path of SNA in the complex plane $(Re(x), Im(x))$ for the acoustic pressure signal obtained at $x_f$ = 17.6 cm, and (b) The corresponding logarithmic plot using differential box-counting algorithm.

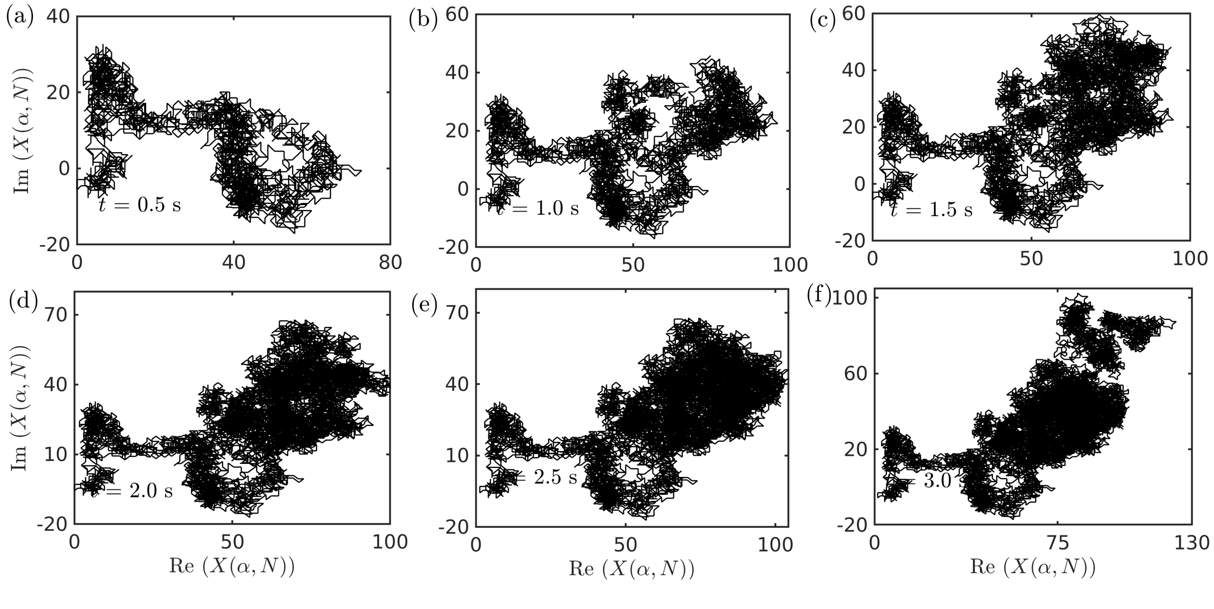


FIG. 2. Spectrum of the SNA in $(Re(x), Im(x))$ plane, for different time scales (a) $t = 0.5s$, (b) $t = 1.0s$, (c) $t = 1.5s$, (d) $t = 2.0s$, (e) $t = 2.5s$, and (f) $t = 3.0s$.
